# Supplementary material for: AutoDistill: an End-to-End Framework to Explore and Distill Hardware-Efficient Language Models
Source: arXiv:2201.08539 source file (2022-01-21)
Supplement: Supplementary file 1 [file sec_appendix.tex]

\section{Please add supplemental material as appendix here}
Put anything that you might normally include after the references as an appendix here, {\it not in a separate supplementary file}. Upload your final camera-ready as a single pdf, including all appendices.
